# Supplementary material for: Generic theory of interacting, spinning, active polar particles: a model for cell aggregates
Source: arXiv:2405.07540 source file (2024-10-31)
Supplement: Supplementary file 1 [file supplementary_material.pdf]

# Supplementary material for : "Generic theory of interacting, spinning, active polar particles: a model for cell aggregates"

Quentin Vagne<sup>1</sup> and Guillaume Salbreux<sup>1</sup>

<sup>1</sup>University of Geneva, Quai Ernest Ansermet 30, 1205 Genève, Switzerland

(Dated: October 31, 2024)

## I. CONSTRAINTS ON PHENOMENOLOGICAL COUPLING COEFFICIENTS

The constraint  $df/dt < 0$  imposes that the symmetric part of the matrix of coupling coefficients (formally described in Eqs.D3,D4 of the main text) must be negative definite. The symmetric part of the matrix of coupling coefficients only includes the dissipative coupling coefficients. Here, they correspond to diagonal terms characterised by  $\Lambda$ ,  $\xi$ ,  $\xi_r$ ,  $\xi'_r$ ,  $\xi_{||}$ ,  $\alpha$ , and non-diagonal terms characterised by  $\Lambda'$ ,  $\beta$ ,  $\beta'$ ,  $\zeta_0$ ,  $\zeta$ ,  $\zeta'$ ,  $\zeta_r$ . Consistently with the simplifications made in the main text, we do not include the coupling coefficients  $\Lambda'$ ,  $\beta$ ,  $\beta'$ . Furthermore, we perform the computation in the illustrative simple case where  $\zeta$ ,  $\zeta'$ ,  $\zeta_r$  are all zero and only  $\zeta_0$  remains. If we arrange the fluxes in the order  $(\mathbf{F}_1^f, \dots, \mathbf{F}_N^f, \mathbf{\Gamma}_1^f, \dots, \mathbf{\Gamma}_N^f, \mathbf{F}_{i_1 j_1}^d, \dots, \mathbf{F}_{i_n j_n}^d, \mathbf{\Gamma}_{i_1 j_1}^d, \dots, \mathbf{\Gamma}_{i_n j_n}^d, D\mathbf{p}_1/Dt, \dots, D\mathbf{p}_N/Dt, r_1, \dots, r_N)$ ,  $n$  being the number of pairs of particles in contact, and the forces in the order  $(\mathbf{v}_1, \dots, \mathbf{v}_N, \mathbf{\Omega}_1, \dots, \mathbf{\Omega}_N, \Delta\mathbf{v}_{i_1 j_1}, \dots, \Delta\mathbf{v}_{i_n j_n}, \mathbf{\Omega}_{i_1} - \mathbf{\Omega}_{j_1}, \dots, \mathbf{\Omega}_{i_n} - \mathbf{\Omega}_{j_n}, -\mathbf{h}_1, \dots, -\mathbf{h}_N, \Delta\mu_1, \dots, \Delta\mu_N)$ , we obtain the following block matrix  $O$ :

$$O = \begin{pmatrix} D_{6(N+n), 6(N+n)} & 0 \\ 0 & M_{4N, 4N} \end{pmatrix}, \quad (1)$$

where  $D_{6(N+n), 6(N+n)}$  is an  $6(N+n) \times 6(N+n)$  diagonal matrix containing  $-\xi$  (repeated  $3N$  times),  $-\xi_r$  (repeated  $3N$  times),  $-\xi_{||}$  (repeated  $3n$  times),  $-\xi'_r$  (repeated  $3n$  times). And the matrix  $M_{4N, 4N}$  is:

$$\begin{pmatrix} -\alpha & 0 & 0 & 0 & 0 & 0 & \dots & A_{p1x} & 0 & \dots & 0 \\ 0 & -\alpha & 0 & 0 & 0 & 0 & \dots & A_{p1y} & 0 & \dots & 0 \\ 0 & 0 & -\alpha & 0 & 0 & 0 & \dots & A_{p1z} & 0 & \dots & 0 \\ 0 & 0 & 0 & -\alpha & 0 & 0 & \dots & 0 & A_{p2x} & \dots & 0 \\ 0 & 0 & 0 & 0 & -\alpha & 0 & \dots & 0 & A_{p2y} & \dots & 0 \\ 0 & 0 & 0 & 0 & 0 & -\alpha & \dots & 0 & A_{p2z} & \dots & 0 \\ \dots & \dots \\ A_{p1x} & A_{p1y} & A_{p1z} & 0 & 0 & 0 & \dots & -\Lambda & 0 & \dots & 0 \\ 0 & 0 & 0 & A_{p2x} & A_{p2y} & A_{p2z} & \dots & 0 & -\Lambda & \dots & 0 \\ \dots & \dots \\ 0 & 0 & 0 & 0 & 0 & 0 & \dots & 0 & 0 & \dots & -\Lambda \end{pmatrix}, \quad (2)$$

where  $\mathbf{A}_{pi} = \zeta_0 \mathbf{p}_i$ . The eigenvalues  $x$  of  $O$  must be negative, and are the solutions of the characteristic polynomial of  $O$ :

$$\det(O - xI_d) = 0. \quad (3)$$

In order to compute the determinant, we make use of the block matrix determinant formula [1]:

$$\det \begin{pmatrix} A & B \\ C & D \end{pmatrix} = \det(A) \det(D - CA^{-1}B). \quad (4)$$

We define  $\tilde{D} = D - xI_d$ ,  $\tilde{M} = M - xI_d$ , and using the block matrix determinant formula we have:

$$\det(O - xI_d) = \det(\tilde{D}) \det(\tilde{M}) = (-\xi - x)^{3N} (-\xi_r - x)^{3N} (-\xi_{||} - x)^{3n} (-\xi'_r - x)^{3n} \det(\tilde{M}). \quad (5)$$

Using the block matrix determinant again on  $\tilde{M}$ , we find:

$$\det(\tilde{M}) = (-\alpha - x)^{2N} \prod_{i=1}^N (x^2 + x(\alpha + \Lambda) + \Lambda\alpha - \mathbf{A}_{pi}^2). \quad (6)$$

From this we have the full list of all the eigenvalues of  $O$ :

$$-\xi, \quad -\xi_r, \quad -\xi_{||}, \quad -\xi'_r, \quad -\alpha, \quad \frac{1}{2} \left( -\Lambda - \alpha \pm \sqrt{\alpha^2 + 4\mathbf{A}_{pi}^2 - 2\alpha\Lambda + \Lambda^2} \right) \forall i \in 1 \dots N. \quad (7)$$

In this paper, we consider the case where the polarities are normalised and the distance between neighbouring particles is equal to  $2R$  with  $R$  the size of the object represented by the particle. Therefore, for a fixed value of  $\zeta_0$ , the  $\mathbf{A}_{pi}^2$  terms are bounded. Provided that the kinetic coefficient  $\Lambda$  linking the reaction rate to the chemical potential difference is large enough and positive, the eigenvalues asymptotically become:

$$-\xi, -\xi_r, -\xi_{||}, -\xi'_r, -\alpha, -\Lambda. \quad (8)$$

This means that (in the case of large  $\Lambda$ ) the only constraints on the coupling coefficients are:

$$\xi > 0, \xi_r > 0, \xi_{||} > 0, \xi'_r > 0, \alpha > 0, \Lambda > 0. \quad (9)$$

## II. EFFECT OF CONFINEMENT ON THE STABILITY OF ROTATING STATES

Phase diagrams shown on Fig.3b,c of the main text show that the stability of steady-states such as the rotating states or the flocking states are strongly impacted by the presence (or absence) of confinement. While rotating states are unstable for a doublet that is free to translate, the addition of a confinement force (described in Appendix F1b of the main text) stabilises them. In the specific case of Fig.3b,c, the only non-zero parameters in the constitutive equations (Eq.18 in the main text) are  $\lambda, \eta, \xi, \xi_r, \xi_{||}$  and  $\alpha$ . In order to obtain an intuitive understanding of this behaviour, we consider the even simpler case of  $\xi_{||} = 0$  and  $\xi_r \rightarrow \infty$ . Since we assume that  $\alpha \rightarrow \infty$ , we have  $\mathbf{h}_i \rightarrow 0$  while  $\alpha \mathbf{h}_i = -2\alpha\kappa_i \mathbf{p}_i$  is adjusted such that the norm of  $\mathbf{p}_i$  is fixed. In the following, we simplify the notations by redefining the Lagrange multipliers such that  $-2\alpha\kappa_i$  is simply written as  $\kappa_i$ , and  $2\kappa_r \mathbf{r}_{12}$  is written as  $\kappa_r \hat{\mathbf{r}}_{12}$  where  $\hat{\mathbf{r}}_{12} = \mathbf{r}_{12}/\|\mathbf{r}_{12}\|$ .

### A. Case without confinement

The equations for the dynamics (Eq. F3 in the main text) become:

$$\begin{aligned} \lambda \mathbf{p}_1 - \xi \mathbf{v}_1 + \kappa_r \hat{\mathbf{r}}_{12} &= 0, \quad \boldsymbol{\Omega}_1 = 0, \quad \frac{d\mathbf{p}_1}{dt} = -\eta \mathbf{v}_1 + \kappa_1 \mathbf{p}_1, \\ \lambda \mathbf{p}_2 - \xi \mathbf{v}_2 - \kappa_r \hat{\mathbf{r}}_{12} &= 0, \quad \boldsymbol{\Omega}_2 = 0, \quad \frac{d\mathbf{p}_2}{dt} = -\eta \mathbf{v}_2 + \kappa_2 \mathbf{p}_2. \end{aligned} \quad (10)$$

In dimensionless units, we have:

$$\begin{aligned} \lambda \mathbf{p}_1 + \kappa_r \hat{\mathbf{r}}_{12} &= \mathbf{v}_1, \quad \boldsymbol{\Omega}_1 = 0, \quad \frac{d\mathbf{p}_1}{dt} = -\eta \mathbf{v}_1 + \kappa_1 \mathbf{p}_1, \\ \lambda \mathbf{p}_2 - \kappa_r \hat{\mathbf{r}}_{12} &= \mathbf{v}_2, \quad \boldsymbol{\Omega}_2 = 0, \quad \frac{d\mathbf{p}_2}{dt} = -\eta \mathbf{v}_2 + \kappa_2 \mathbf{p}_2. \end{aligned} \quad (11)$$

The dimensionless versions of  $\lambda, \eta$  stand for  $\lambda/|\lambda| = \pm 1$  and  $\eta R$ . The dimensionless velocities  $\mathbf{v}_i$  stand for  $\xi \mathbf{v}_i/R$ . The constraint  $(\mathbf{v}_2 - \mathbf{v}_1) \cdot \hat{\mathbf{r}}_{12} = 0$  can be used to compute  $\kappa_r$ , and then the force balance equations provide the expressions of the velocities:

$$\mathbf{v}_1 = \lambda \mathbf{p}_1 - \frac{\lambda}{2} [(\mathbf{p}_1 - \mathbf{p}_2) \cdot \hat{\mathbf{r}}_{12}] \hat{\mathbf{r}}_{12}, \quad \mathbf{v}_2 = \lambda \mathbf{p}_2 - \frac{\lambda}{2} [(\mathbf{p}_2 - \mathbf{p}_1) \cdot \hat{\mathbf{r}}_{12}] \hat{\mathbf{r}}_{12}. \quad (12)$$

From the velocities, we get the rotation of the unit vector  $\hat{\mathbf{r}}_{12}$ :

$$\frac{d\hat{\mathbf{r}}_{12}}{dt} = \frac{1}{2}(\mathbf{v}_2 - \mathbf{v}_1) = \boldsymbol{\Omega}_d \times \hat{\mathbf{r}}_{12}, \quad (13)$$

where  $\|d\hat{\mathbf{r}}_{12}/dt\| = \|\boldsymbol{\Omega}_d\|$  is the rate at which the doublet rotates. A steady-state is observed if, in a reference frame following  $\hat{\mathbf{r}}_{12}$ , there is no motion of the polarities  $\mathbf{p}_i$ . This is the case if  $d\mathbf{p}_i/dt = \boldsymbol{\Omega}_d \times \mathbf{p}_i$ . We therefore define a co-rotating polarity evolution  $\delta \mathbf{p}_i / \delta t = d\mathbf{p}_i / dt - \boldsymbol{\Omega}_d \times \mathbf{p}_i$ , the dynamics of which is:

$$\frac{\delta \mathbf{p}_i}{\delta t} = -\boldsymbol{\Omega}_d \times \mathbf{p}_i - \eta \mathbf{v}_i + \kappa_i \mathbf{p}_i, \quad \text{with } \|\boldsymbol{\Omega}_d \times \mathbf{p}_i\| = \|\boldsymbol{\Omega}_d\| = \left\| \frac{1}{2}(\mathbf{v}_2 - \mathbf{v}_1) \right\|, \quad (14)$$

where we call  $-\boldsymbol{\Omega}_d \times \mathbf{p}_i$  the co-rotation term. In Fig.1, we first use Eq. 12 to compute the velocities as a function of the polarities  $\mathbf{p}_i$ . Then we use Eq. 14 to compute the co-rotating polarity evolution.

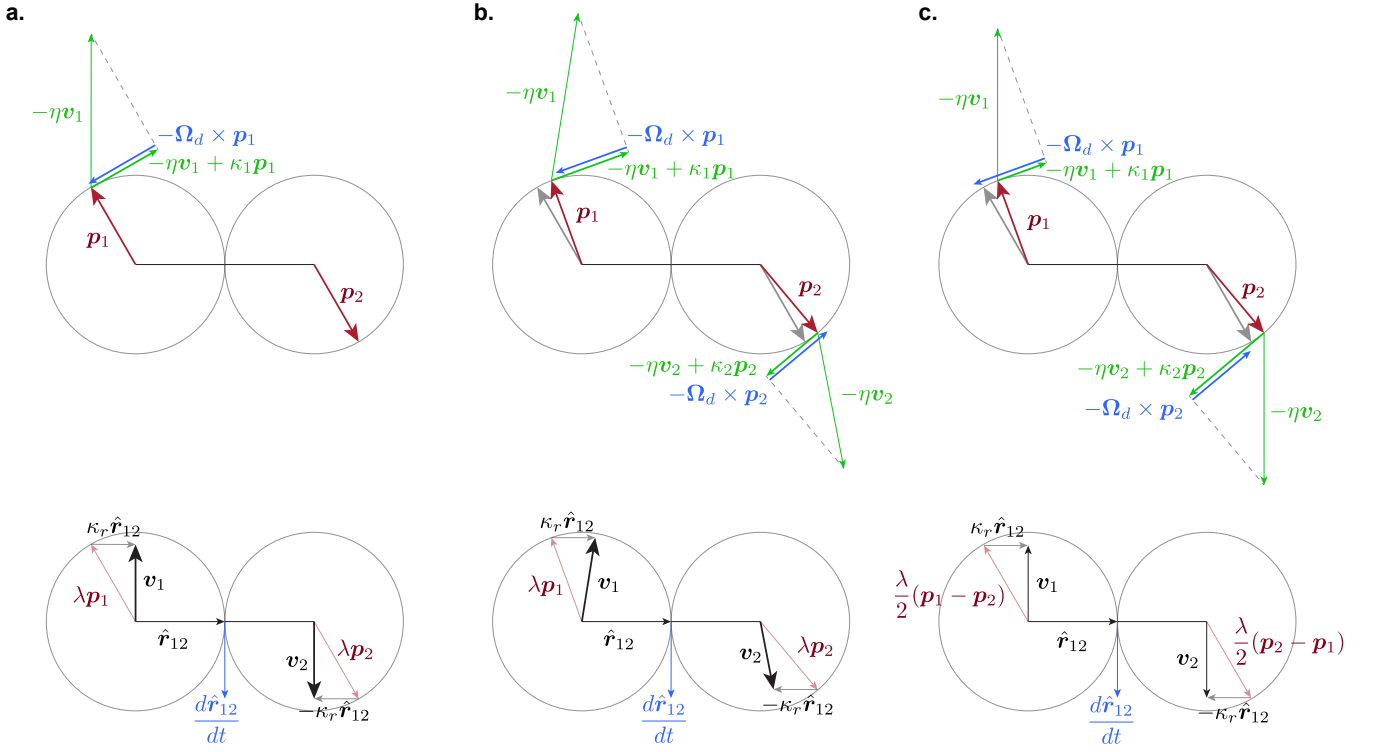

Supplementary Figure 1: Effect of confinement on the rotating state ( $\Delta\psi_1 = 2\pi/3$ ,  $\Delta\psi_2 = -\pi/3$ ) for  $\lambda = +1$ ,  $\eta = -2$ . The top panel shows the polarity orientations and their dynamics, controlled by flow alignment ( $-\eta\mathbf{v}_i$ ) and doublet rotation ( $-\mathbf{\Omega}_d \times \mathbf{p}_i$ ). The bottom panel shows the velocities  $\mathbf{v}_i$  (and the term  $d\hat{\mathbf{r}}_{12}/dt = \mathbf{\Omega}_d \times \hat{\mathbf{r}}_{12}$  characterising doublet rotation), emerging from self-propulsion ( $\lambda\mathbf{p}_i$ ) and the constraint of fixed radius ( $\kappa_r\hat{\mathbf{r}}_{12}$ ). a: Rotating steady-state, where the flow alignment exactly compensates the drift due to doublet rotation. b: Slightly perturbed state ( $\delta\Delta\psi_1 < 0$ ,  $\delta\Delta\psi_2 > 0$ ), without confinement. c: Same perturbation, with confinement.

## B. Case with confinement

In the case of confinement, an external force  $\mathbf{F}_{\text{ext}}$  is added in the force balance in order to enforce the constraint  $\mathbf{v}_1 + \mathbf{v}_2 = 0$ :

$$\begin{aligned}\lambda\mathbf{p}_1 + \kappa_r\hat{\mathbf{r}}_{12} + \mathbf{F}_{\text{ext}} &= \mathbf{v}_1, \\ \lambda\mathbf{p}_2 - \kappa_r\hat{\mathbf{r}}_{12} + \mathbf{F}_{\text{ext}} &= \mathbf{v}_2.\end{aligned}\tag{15}$$

We find  $\mathbf{F}_{\text{ext}} = -\lambda/2(\mathbf{p}_1 + \mathbf{p}_2)$ , which leads to the following modified expressions of the velocities:

$$\mathbf{v}_1 = \frac{\lambda}{2}(\mathbf{p}_1 - \mathbf{p}_2) - \left[ \frac{\lambda}{2}(\mathbf{p}_1 - \mathbf{p}_2) \cdot \hat{\mathbf{r}}_{12} \right] \hat{\mathbf{r}}_{12}, \quad \mathbf{v}_2 = \frac{\lambda}{2}(\mathbf{p}_2 - \mathbf{p}_1) - \left[ \frac{\lambda}{2}(\mathbf{p}_2 - \mathbf{p}_1) \cdot \hat{\mathbf{r}}_{12} \right] \hat{\mathbf{r}}_{12}.\tag{16}$$

The polarity dynamics is unchanged, given by Eq. 14.

## C. Stability of the rotating state

We now consider the case  $\eta = -2$ , for which the rotating steady-state exists (with or without confinement) with  $\Delta\psi_1 = 2\pi/3$  and  $\Delta\psi_2 = -\pi/3$ . In this case, we see on Supplementary Figure 1a that the co-rotation term balances exactly the flow alignment term. However, when a small perturbation is introduced on the polarities (Supplementary Figure 1b-c) the individual velocities change due to the self-propulsion force, and the flow alignment terms are not compensated any more by the co-rotation terms. Without confinement, a slight translational motion of the doublet appears, which exacerbates the perturbation, showing that the rotating state is unstable (Supplementary Figure 1b). In the presence of confinement (Supplementary Figure 1c), the translational motion of the doublet is cancelled, such that the cell velocities remain perpendicular to  $\hat{\mathbf{r}}_{12}$ , which then changes the flow alignment terms and affects the polarity dynamics. We see in that case that the perturbation shrinks, illustrating that the rotating state is stabilised.

### III. TUMBLING REGIMES

In this section, we discuss the regimes observed in the white regions of Figs. 3,4 in the main text. In these regions, all the steady-states identified using the method described in Appendix F 2 of the main text are either unstable (at least one strictly positive eigenvalue) or marginal (one eigenvalue that is zero). This leads to non-steady trajectories. We characterise the motion using the term “tumbling”, as the motion observed is reminiscent of the run and tumble behaviour of certain bacteria. We discuss separately the tumbling behaviour in Fig.3, which is non deterministic, and arises because of a degenerate mirroring steady-state with a zero eigenvalue, and the behaviour in Fig.4, which is deterministic and periodic.

#### A. Random tumbling, Figure 3

In the case, the tumbling region corresponds to  $\lambda' > 0$  and  $0 < \eta < 1/2$  or  $\lambda' < 0$  and  $-1/2 < \eta' < 0$ . In this region the rotating steady-state is unstable. For the mirroring state, we have  $\Delta\psi_2 = \pi - \Delta\psi_1$ , and we can show (using Eq. F15 in the main text) that any angle  $\Delta\psi_1$  is a solution. This shows that the state is degenerate, and that one of the eigenvalue will always be zero. Indeed, for the eigenvalues, we find, as a function of  $\Delta\psi_1$ :

$$0, \frac{4}{5}\lambda' \cos(\Delta\psi_1)(2\eta' \cos(\Delta\psi_1) + 1). \quad (17)$$

For the values of  $\Delta\psi_1$  for which the second eigenvalue stays negative, the doublet will remain in a mirroring state, but the angle  $\Delta\psi_1$  will be free to diffuse, in the presence of even a small amount of noise. If the second eigenvalue becomes positive, however, the mirroring state will become unstable, leading to a tumbling motion. We can check mathematically from Eq. 17 that, for any value of  $\eta'$ ,  $\lambda'$ , there exists always a real  $\Delta\psi_1$  for which the second eigenvalue is positive. This means that in the presence of noise, from the mirroring state the doublet will always become unstable at some point and execute a tumble. In the white region of the phase diagram of Fig.3, no other state is stable so after tumbling the doublet will end up in a mirroring state again, from which it will repeat the cycle. In order to observe this dynamic, we introduce a noise term in the equations of motions:

$$\begin{aligned} \frac{d\Delta\psi_1}{dt} &= \frac{2}{5}\lambda'(1 + 2\eta' \cos(\Delta\psi_1))(\sin(\Delta\psi_1) - \sin(\Delta\psi_2)) + \sigma_1, \\ \frac{d\Delta\psi_2}{dt} &= \frac{2}{5}\lambda'(-1 + 2\eta' \cos(\Delta\psi_2))(\sin(\Delta\psi_2) - \sin(\Delta\psi_1)) + \sigma_2, \\ \frac{d\theta}{dt} &= -\frac{1}{5}\lambda'(\sin(\Delta\psi_1) - \sin(\Delta\psi_2)), \end{aligned} \quad (18)$$

Where  $\sigma_i$  are Gaussian noises such that  $\langle \sigma_i(t)\sigma_j(t') \rangle = \sigma\delta_{ij}\delta(t-t')$ . An example of a time course of such a simulation is shown on Supplementary Figure 2a. It shows an alternating phases of diffusion where  $\Delta\psi_1$  and  $\Delta\psi_2$  stay the mirror of one another but slowly drift, and very short phases of tumbling where the doublet rapidly rotates until it settles into a new mirroring state.

#### B. Deterministic run and tumbles, Figure 4

In the phase diagram of Fig.4a of the main text, in the white region, all steady-states are unstable and there is no degeneracy. The equations of motions for  $\Delta\psi_1$ ,  $\Delta\psi_2$  are (from Eq.F16 in the main text):

$$\begin{aligned} \frac{d\Delta\psi_1}{dt} &= \frac{1}{10}(-20\zeta_{rp} \sin(2\Delta\psi_1) + (\lambda - 20)\sin(\Delta\psi_1) - \lambda \sin(\Delta\psi_2)), \\ \frac{d\Delta\psi_2}{dt} &= \frac{1}{10}(\lambda \sin(\Delta\psi_1) - \sin(\Delta\psi_2)(40\zeta_{rp} \cos(\Delta\psi_2) + \lambda - 20)). \end{aligned} \quad (19)$$

Solving for these equations numerically allows to obtain  $\Delta\psi_1(t)$  and  $\Delta\psi_2(t)$ , from which we can compute the full trajectory of the doublet, characterised by  $\theta(t)$  and the center of mass coordinates  $x(t)$ ,  $y(t)$ , by integrating the

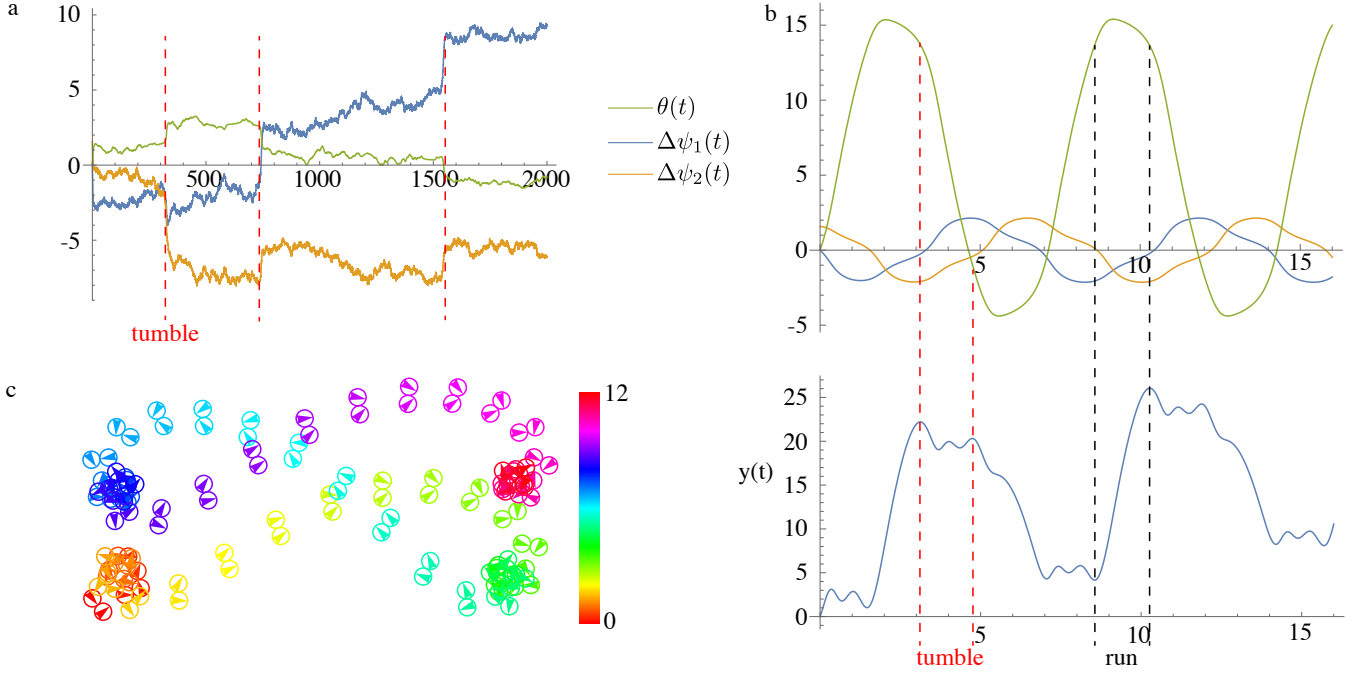

Supplementary Figure 2: Time traces of tumbling simulations, with red lines indicating moments of "tumbles", and black lines indicating moments of "run". a,b(top): Time evolution of the angles  $\theta(t)$ ,  $\Delta\psi_1(t)$ ,  $\Delta\psi_2(t)$ , defined on Fig.2a of the main text, for two different cases of tumbling: a: Random tumbling, as on Fig.3 of the main text, obtained by solving Eq. 18. 2000 dimensionless time units are shown for a simulation made with  $\sigma = 0.1$ ,  $\lambda' = 1$ ,  $\eta' = 0.2$ . b: Deterministic tumbling, as on Fig.4 of the main text, obtained by solving Eqs.19,20 with  $\lambda = 20$ ,  $\zeta_{rp} = -1/2$ . The bottom curve shows the motion along  $y$  of the doublet center of mass. c: Trajectory of the doublet in the 2D space, corresponding to the simulation in b. The color represents time.

following equations:

$$\begin{aligned}
 \frac{d\theta}{dt} &= -\frac{3}{10}\lambda(\sin(\Delta\psi_1) - \sin(\Delta\psi_2)) , \\
 \frac{dx}{dt} &= \frac{\lambda}{2}(\cos(\theta + \Delta\psi_1) + \cos(\theta + \Delta\psi_2)) , \\
 \frac{dy}{dt} &= \frac{\lambda}{2}(\sin(\theta + \Delta\psi_1) + \sin(\theta + \Delta\psi_2)) .
 \end{aligned} \tag{20}$$

An example of trajectory is shown on Supplementary Figure 2 b,c. We see that the evolution is typically periodic in terms of  $\Delta\psi_1$ ,  $\Delta\psi_2$ ,  $\theta$ , but not in terms of center of mass motion. There is a constant translation after each period. We also notice alternating phases of 'tumbling' where the doublet rotates but does not translate much, and phases of 'run' where the doublet moves in a relatively straight manner without rotating much.

#### IV. CELL-CELL FRICTION INFLUENCE ON ROTATING STATE STABILITY

In the context of rotation from active propulsion and polarity remodelling (described in Appendix E 3 in the main text) there are stable rotating states (main text, blue region in the phase diagram of Fig. 4a, reproduced on Supplementary Figure 3a). These rotating states become unstable when the self-propulsion term becomes large in absolute value. The influence of cell-cell friction on the stability of the rotating states can be made clear by computing a phase diagram (shown on Supplementary Figure 3b) as a function of self-propulsion and the ratio  $\xi_{||}R^2/\xi_r$  of cell-cell friction over rotational friction. As the cell-cell friction becomes larger, the threshold value of  $\lambda$  above which the rotating state becomes unstable increases, and the cell intrinsic rotation rate  $\Omega$  approaches the doublet rotation rate  $\Omega_d$ , such that the doublet rotates asymptotically as a solid object.

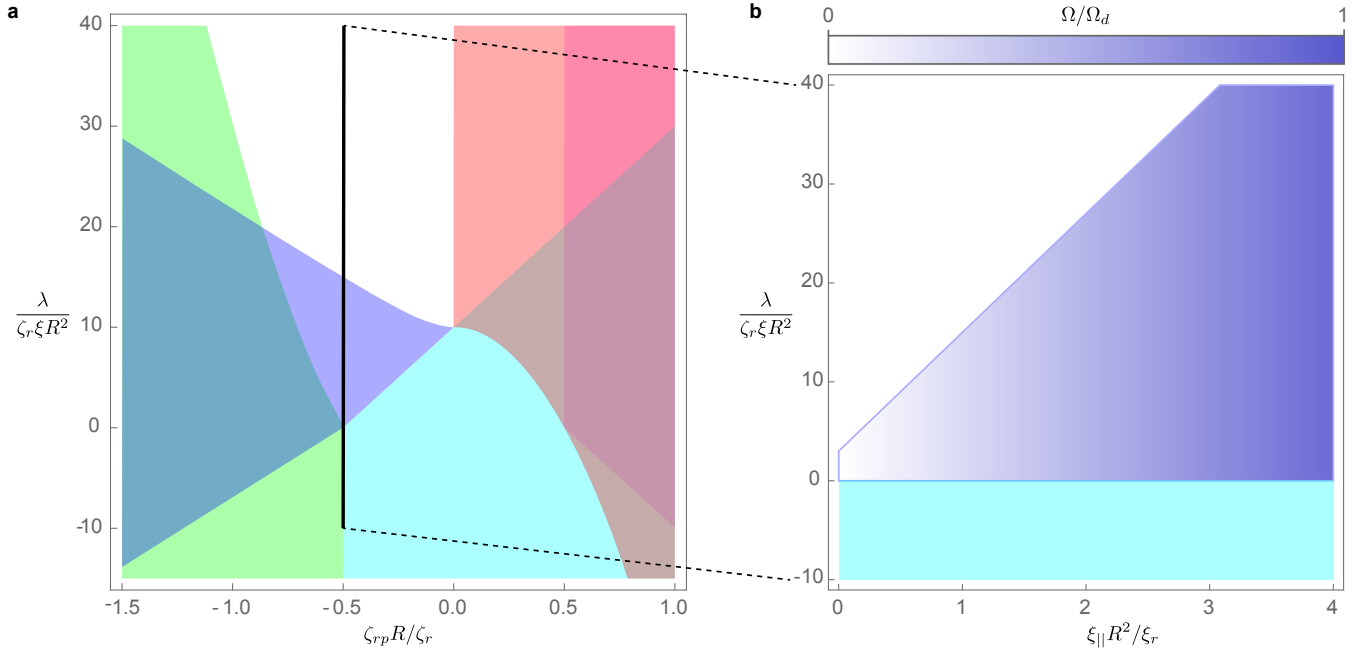

Supplementary Figure 3: **a**: Phase diagram from Fig. 4a of the main text, with  $\xi_{||} R^2 / \xi_r = 1$ . The black line shows a cut at  $\zeta_{rp} R / \zeta_r = -1/2$ , for which we study the effect of cell-cell friction vs rotational friction, in panel b. **b**: Phase diagram as a function of self-propulsion  $\lambda / (\zeta_r \xi R^2)$  and ratio of friction coefficients  $\xi_{||} R^2 / \xi_r$ , for  $\zeta_{rp} R / \zeta_r = -1/2$ .  $\Omega$ : individual cell rotation rate,  $\Omega_d$ : doublet rotation rate. Dark blue regions: stable rotating states, clear blue regions: stable 'in' states.

[1] K. M. Abadir and J. R. Magnus, *Matrix Algebra*, Econometric Exercises (Cambridge University Press, 2005).
